# Supplementary material for: A Survey on Deep Learning and Explainability for Automatic Report Generation from Medical Images
Source: arXiv:2010.10563 source file (2022-01-08)
Supplement: Supplementary file 1 [file models-by-paper.tex]

In Table \ref{table:models-by-paper} a summary of each model is presented.

\todo{eliminar esta tabla, o bien pasarla a latex}

\begin{figure}
    \centering
    \includegraphics[width=\textwidth]{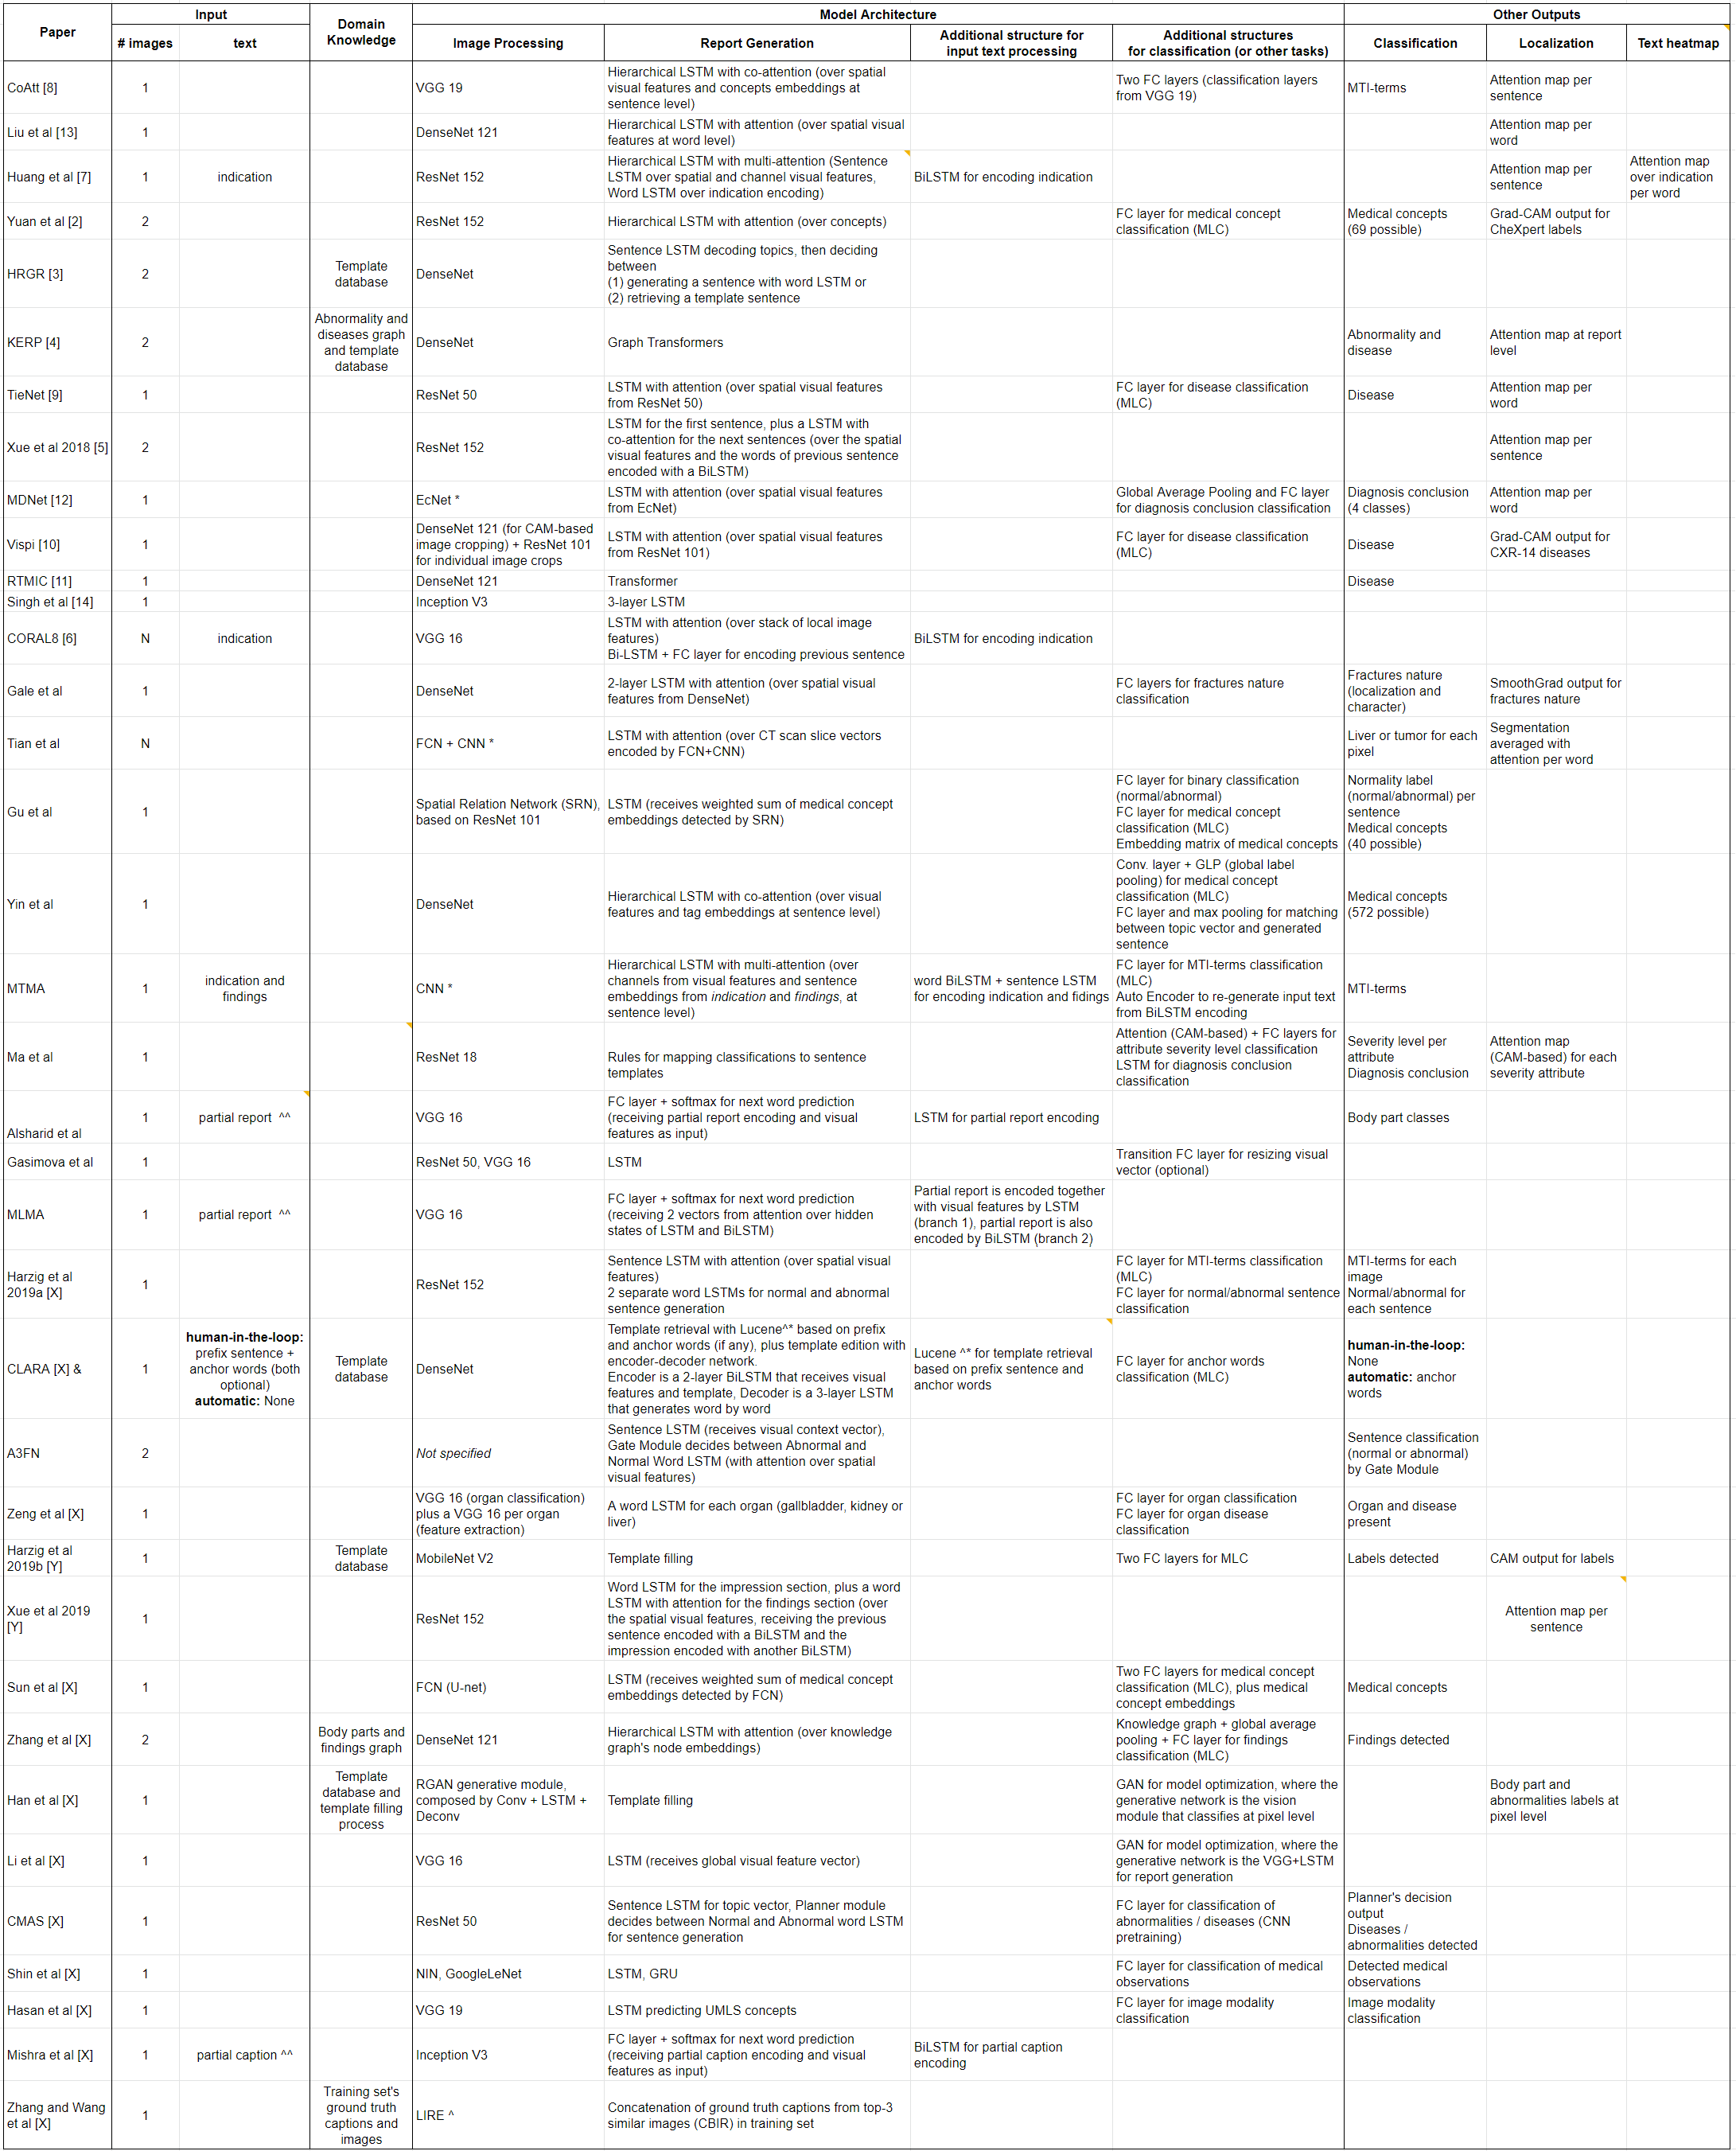}
    \caption{Summary of model architectures in the literature. Best viewed in PDF with zoom.
    (*) ad-hoc architecure.
    LIRE (\^{}) is a library for extracting traditional visual features such as color histograms, texture features, etc (non-DL).
    Lucene (\^{} *) is a software package for text-based information retrieval.
    (\^{}\^{}) These models re-read what they have generated so far to predict the next word (complexity $O(N^2)$, where $N$ is the length of the final report).
    CLARA (\&) has two versions: \textit{human-in-the-loop}, and \textit{automatic}; when unspecified, the entry is valid for both versions.
    Hierarchical LSTM refers to one LSTM for sentences, and one for words.
    LSTM alone generates a full report word by word.
    \textit{indication} is a free text indicated by the physician requesting the imaging exam, while \textit{findings} is the section of the report describing findings in the image.
    \textit{template database} is a set of template sentences, arranged in a specific way.
    MLC stands for Multi-Label Classification, FCN stands for Fully Convolutional Network, and FC stands for Fully Connected.
    }
    \label{table:models-by-paper}
\end{figure}
