# Supplementary material for: A Survey on Deep Learning and Explainability for Automatic Report Generation from Medical Images
Source: arXiv:2010.10563 source file (2022-01-08)
Supplement: Supplementary file 2 [file text-metrics.tex]

In this section, text metrics are explained in further detail, namely BLEU \cite{papineni2002bleu}, ROUGE \cite{lin-2004-rouge}, METEOR \cite{banerjee2005meteor, denkowski2014meteor}, CIDEr \cite{vedantam2015cider} and SPICE \cite{10.1007/978-3-319-46454-1_24}.

Bilingual evaluation understudy (BLEU) \cite{papineni2002bleu} evaluates n-gram overlaps from a target text with one or more ground truth texts.
For a specific value of $n$, BLEU-n can be calculated, such as BLEU-1 for unigrams, BLEU-2 for bigrams, etc; and BLEU is the geometric average of multiple $n$ values.
For both BLEU and BLEU-n the values vary from 0 being the worst to 1 being the best possible value.
All the BLEU variants are oriented to precision and not recall, which means it measures how consistent is the generated report with the ground truth, but not how much information is being captured or being left out.
Nonetheless, the calculation includes a penalization for short sentences.
In the papers reviewed, usually BLEU-n for $n \in \{1, 2, 3, 4\}$ are computed.

Lin \cite{lin-2004-rouge} presented Recall-Oriented Understudy for Gisting Evaluation (ROUGE), which is a set of metrics to assess text similarity, namely ROUGE-N, ROUGE-L, ROUGE-W and ROUGE-S.
For a given $n$ value, ROUGE-$n$ is a recall measure of $n$-grams between the target and reference texts.
ROUGE-L is based on measuring the longest common sub-sequence between the generated and ground truth texts, and it has parameter to bias the metric towards precision, recall, or an average of both (F-score).
ROUGE-W is a modification of ROUGE-L, by adding a weight to favor the sub-sequences with more consecutive words.
Lastly, ROUGE-S measures the co-ocurrences of skip-bigrams, which are bigrams that may have gaps of words, and the calculation can also be inclined for precision, recall or F-score.
In the works reviewed, ROUGE-L is the variant used.

Metric for Evaluation of Translation (METEOR) \cite{banerjee2005meteor, 10.5555/1626355.1626389} focus on finding uni-gram matches between the candidate and reference sentences.
The score is proposed as an F-score inclined towards recall, and it includes a penalization to consider matching longer phrases.
The rules for uni-gram matching incorporate stemming and WordNet \cite{wordnet1995} synonymy, though they are flexible to remove or add more rules.
The same authors expanded the metric \cite{10.5555/1857999.1858030, 10.5555/2132960.2132969, denkowski2014meteor} to facilitate the use of different languages, such as Spanish, and optimizing the hyper-parameters to correlate better with human judgement.
The most updated version seems to be METEOR universal \cite{denkowski2014meteor}.
In the papers reviewed, most of the times is not clear which variant or hyper-parameters were used.

Consensus-based Image Description Evaluation (CIDEr) \cite{vedantam2015cider} is a metric designed to measure the similarity of sentences in terms of the n-grams forming them.
Specifically, it represents each sentence with a TF-IDF score over the n-grams, where the term-frequency measures the presence of each n-gram in the sentence, and the inverse-document-frequency part gives less importance to the most frequent n-grams in the dataset, assuming those will provide less valuable information.
Then, the likeness between two sentences is calculated as the cosine similarity between the two vectors from each one.
As usual, the metric can be calculated for a given $n$ value, as CIDEr$_n$, or as an average of multiple $n$ values summed up as CIDEr.
Also, the authors presented a variant more robust against gameability, CIDEr-D.
% , although the most common variant used in the papers reviewed is the original CIDEr.
The authors argue that with this measure of similarity both precision and recall are being captured, and by using multiple $n$ values, grammatical and semantic notions are preserved.

Semantic Propositional Image Caption Evaluation (SPICE) \cite{10.1007/978-3-319-46454-1_24} is proposed as an image captioning metric, and is designed to evaluate the underlying meaning of the sentences describing the scene, disregarding fluency or grammar aspects.
To this end, the semantic information is captured by parsing a caption to a graph representing the objects in the scene, relations between them and their attributes.
Then, two captions have a similar meaning if their graphs are similar, thus, a matching between the target caption graph and ground truth's graph is computed, and SPICE is calculated as an F-score.
Similar to METEOR, lemmatization and WordNet \cite{wordnet1995} synonymy are included to further improve the semantic matching.
The authors reported better correlation with human judgement than BLEU, ROUGE-L, METEOR and CIDEr, though they acknowledge the need of an alternative metric measuring syntactic aspects to use in tandem with SPICE.
Although this text quality metric is essentially different from the previously described, which are mainly based on n-gram matching, we believe that the original SPICE is still not suitable for medical domain reports, as the objects, relations and attributes differ significantly from those in the general domain.
Li et al \cite{10.1145/3357254.3357256} is the only work that uses SPICE, but the concepts and attributes used for the computation are not specified, thus we label this metric as a general text quality method, and not as medical correctness.
